# Supplementary material for: The Diamond (111) Surface Reconstruction and Epitaxial Graphene Interface
Source: arXiv:2202.09151 source file (2022-02-21)
Supplement: Supplementary file 1 [file Diamond_111_Supp.pdf]

# Supplemental Material
# The diamond (111) surface reconstruction and epitaxial graphene interface

B. P. Reed,[1, 2, 3] M. E. Bathen,[4, 5] J. W. R. Ash,[1, 2] C. J. Meara,[6]
A. A. Zakharov,[7] J. Goss,[6] J. W. Wells,[5] D. A. Evans,[1] and S. P. Cooil[1, 5, *]

[1] *Department of Physics, Aberystwyth University, Aberystwyth, SY23 3BZ, United Kingdom.*
[2] *Centre for Doctoral Training in Diamond Science and Technology, University of Warwick, Coventry, CV4 7AL, United Kingdom.*
[3] *National Physical Laboratory, Teddington, TW11 0LW, United Kingdom.*
[4] *Advanced Power Semiconductor Laboratory, ETH Zurich, Physikstrasse 3, Zurich, 8092, Switzerland.*
[5] *Centre for Materials Science and Nanotechnology, University of Oslo, Oslo, 0318, Norway.*
[6] *School of Electrical and Electronic Engineering, Newcastle University, Newcastle-upon-Tyne, UK, NE1 7RU, United Kingdom.*
[7] *Max IV Laboratory, Lund University, Lund, 221 00, Sweden.*

(Dated: February 18, 2022)

## I. TEMPERATURE CALIBRATION

In the Aberystwyth real-time electron emission spectroscopy (REES) system, calibration of the sample temperature relative to the k-type thermocouple located on the substrate heater is performed by non-contact methods. This is achieved by comparison of the measured thermocouple temperature $T$ to that calculated by the temperature dependence of the first order phonon line of diamond $\Omega\,(T)$ using (1),

$$\Omega\,(T) = \Omega_0 - \frac{C}{e^{\left[D\left(\frac{hc\Omega_0}{kT}\right)\right]} - 1} \tag{1}$$

where the position of the first order phonon line at 0 K is $\Omega_0$ =1332.7 cm$^{-1}$. Here, $C$ and $D$ are free parameters used to fit the experimental data of Zouboulis and Grimsditch [1] and of Solin and Ramadas [2] with values of 61.14 cm$^{-1}$ and 0.787 respectively, as detailed in Refs [3, 4]. Snapshots of the main diamond line were recorded every 9 s (3×3 s integration) during the heating cycle. The results are presented in Fig. S1(a) and (b).

In our set up a Horiba LabRam HR800 is fibre-coupled to a "Superhead" lens system mounted on the ambient side of the UHV system's window, as shown in Fig. S1(c). The Superhead delivers laser light and collects the Raman shifted light through a ×10 microscope objective and telescopic lens allowing for a variable focal length of ≈250 to 400 mm. Inside the Superhead there are notch and edge filters present for cleaning the input beam and removing the main laser line from the measurement signal, respectively. The collected light is guided back to the Peltier cooled spectrometer via a 400 µm optical fibre. The inset in Fig. S1(c) shows the location of the k-type thermocouple relative to the sample.

## II. THE C(111)-(1 × 1):H SURFACE

Angle-resolved photoemission spectroscopy (ARPES) was performed on the H-terminated diamond surface to investigate the position of the valence band maximum prior to surface reconstruction and subsequent graphene formation. The sample was initially H-terminated as described in the main text and then degassed in vacuo at 300 °C. The results are presented in Fig. S2. The value of the valence band maximum at $E_\mathrm{B} = 0.66$ eV used to place the calculated $\sigma$-band maximum is referenced to the peak position of the energy dispersive cut (EDC) shown in Fig. S2(c) extracted at $\bar{\Gamma}$ from the second differential image presented inhttps://www.overleaf.com/project/61701fdf48ec2358e16cdb37 Fig. S2(b).

* Corresponding author email: scooil@icloud.com;
Current address: Centre for Materials Science and Nanotechnology, University of Oslo, Oslo, 0318, Norway.

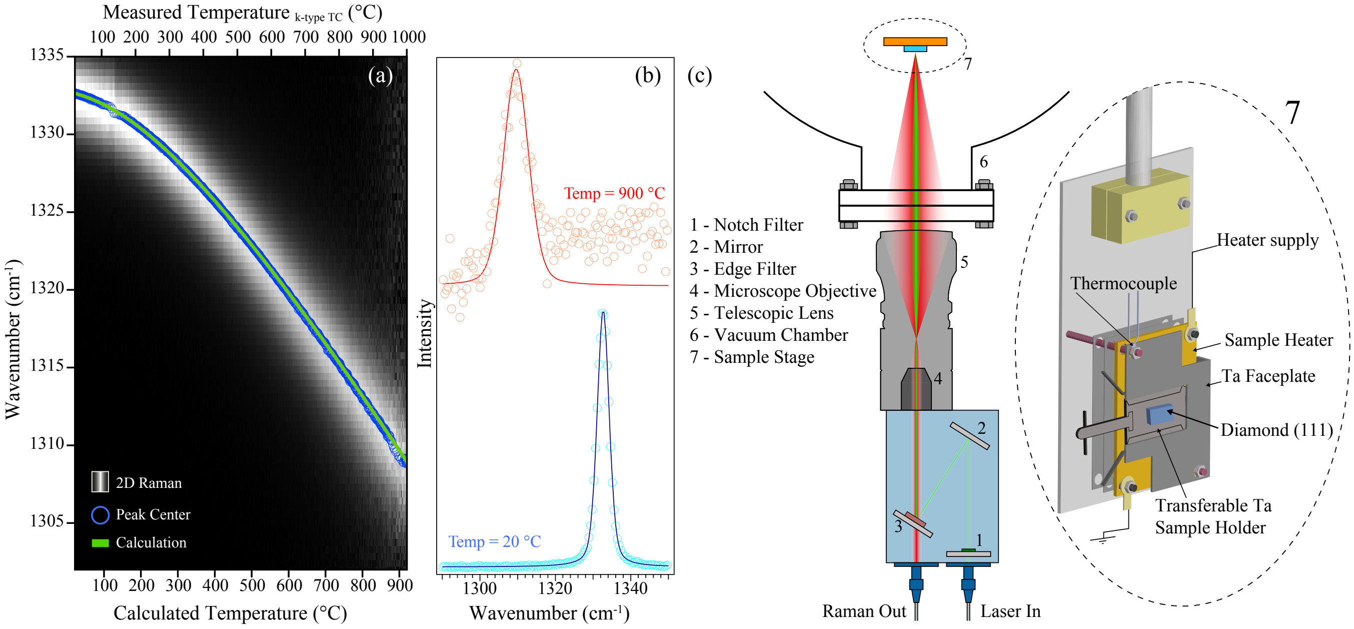


FIG. S1. Temperature dependent Raman shift of the main phonon line from a single crystal diamond (111) sample. (a) Displays the 2D dataset of the main phonon line vs measured temperature with the peak centre plotted as open blue circles. The green solid line is the calculated shift using the parameters extracted from Refs. [3, 4]. (b) Raman signals extracted from the 2D dataset at 20 °C and 900 °C, the measured data is shown as open circles and the fit as a solid line in blue and red respectively. (c) Schematic diagram of the Raman Superhead system and sample stage detailing the location of the thermocouple relative to the sample.

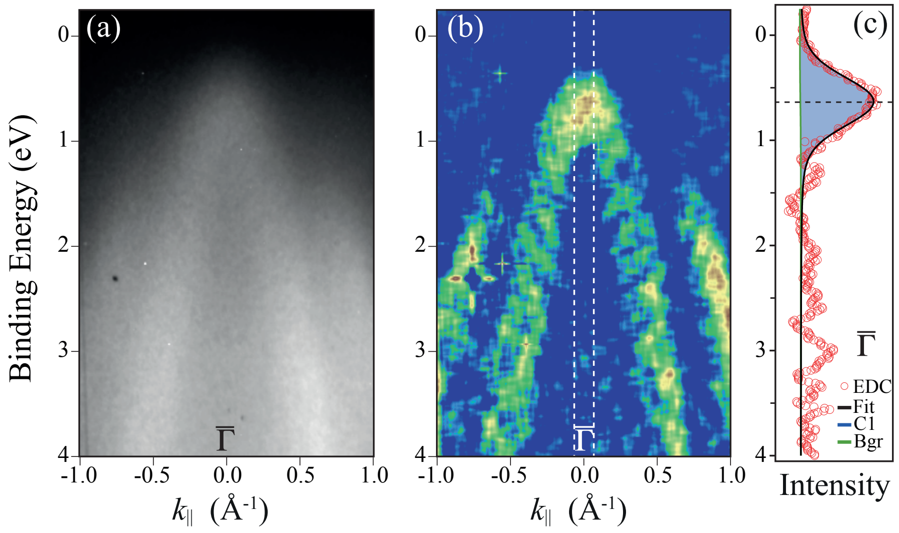


FIG. S2. Photoemission intensity of the $\sigma$-bands nearest the $E_F$ for the C(111)-(1 × 1):H surface. (a) The measured intensity from the ARPES experiment. (b) Two-dimensional 2nd differential image of the data. The image is formed from the sum of 2nd differentials taken in the momentum dispersive direction (MDCs) and the energy dispersive direction (EDCs), boxcar smoothing of 5 pixels in each direction has been performed. (c) EDC taken at $\bar{\Gamma}$ from a region of $k_{\parallel} = 0.1\,\text{Å}^{-1}$ wide, the red open circles show the intensity, the black solid line is the result of fitting one Voigt component, C1, centred at $E_B = 0.66\,\text{eV}$ shown in pale blue and a Shirley-like background subtraction shown as the green solid line.

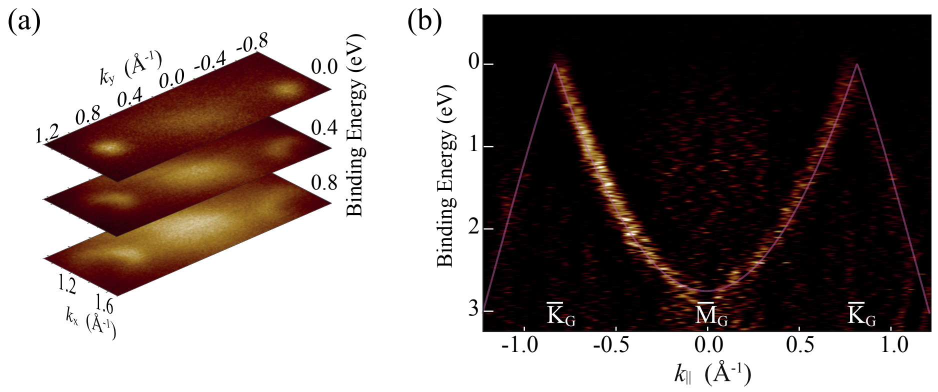


FIG. S3. Photoemission intensity of the graphene $\pi$-band along the $\overline{K}_G$-$\overline{M}_G$-$\overline{K}'_G$ edge of graphene's BZ. (a) Constant energy surfaces showing the triangular modulation of the photoemission intensity characteristic of graphene. (b) Two dimensional differential image of the dispersion presented in Fig. 3(c) in the main text. The second differential is used to enhance the weak intensity of the band as it continues towards the next graphene zone center $\overline{\Gamma}'$. Overlayed as the magenta solid line on the figure is the bare band DFT calculation as detailed in the main text.

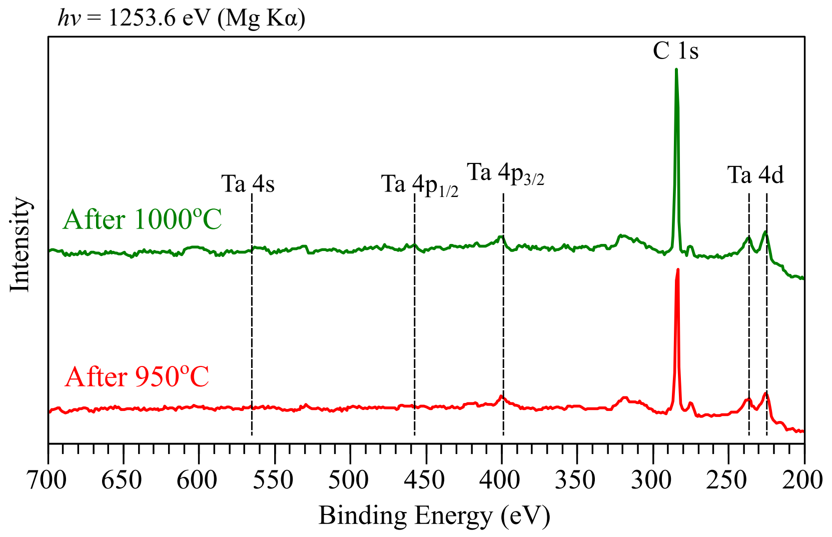


FIG. S4. Widescan XPS measurements collected at a pass energy of 100 eV and $h\nu$ = 1253.6 eV after 950 °C and 1000 °C respectively on the type-Ia diamond substrate. Due to the small size of the diamond sample, the 'Small Area' lens mode of the Specs PHOIBOS 100 was used, therefore extended acquisition times were required to achieve an acceptable signal-to-noise. Regardless, tantalum from the sample holder was still detected in the widescans. As evidenced by Fig. 4 in the main text, there are no adventitious carbon or carbide components from the tantalum that contribute to the C 1s signal.

[1] E. S. Zouboulis and M. Grimsditch, Raman scattering in diamond up to 1900 K, Phys. Rev. B **43**, 12490 (1991).
[2] S. A. Solin and A. K. Ramdas, Raman spectrum of diamond, Phys. Rev. B **1**, 1687 (1970).
[3] J. B. Cui, K. Amtmann, J. Ristein, and L. Ley, Noncontact temperature measurements of diamond by raman scattering spectroscopy, J. Appl. Phys. **83**, 7929 (1998).
[4] M. S. Liu, L. A. Bursill, S. Prawer, and R. Beserman, Temperature dependence of the first-order raman phonon line of diamond, Phys. Rev. B **61**, 3391 (2000).
